# Supplementary material for: Task load dependent decision referrals for joint binary classification in human-automation teams
Source: arXiv:2504.04248 source file (2025-04-05)
Supplement: Supplementary file 1 [file appendix.tex]

\section{Appendix}
\subsection{Experiment Design }
We will now describe our experimental design using standard terminology \cite{Oehlert:book2010:FCDAE, Montgomery:book2017:DAE}. 
\begin{enumerate}
    \item \textit{Experimental units --- } Individual human participants (who have volunteered to take part in the study).
    \item \textit{Treatments ---}
    Allocation policies used to refer decisions to the humans. In the first experiment the treatments applied are optimal allocation and random allocation schemes under fixed workloads. In the second experiment the treatments applied are optimal allocation and blind allocation.

    \item \textit{Statistical Hypothesis testing ---} The two competing hypotheses being tested in the experiment are whether both the treatments (task allocation schemes) are equivalent or the optimal allocation scheme is better. This comparison can be done in terms of the mean costs and variances of costs achieved by both treatments. The statistical model for the data is as follows. For $n$ experimental units, 
    \begin{align}
        y^B_j = m_B  + {\epsilon}^B_j + \beta_j,\nonumber\\
        y^O_j = m_O  + {\epsilon}^O_j + \beta_j,\nonumber\\ 
        j=1,2,\ldots,n,
    \end{align}
    where $[y^B_j]_{j=1:n}$ and $[y^O_j]_{j=1:n}$ are vectors containing sample batch costs for blind allocation and optimal allocation schemes, respectively. Also, $m_B$ and $m_O$ are the true mean costs of these groups. ${\epsilon}^B_j$ and ${\epsilon}^O_j$ are random experimental errors with zero means and variances $v^B,v^O.$ These random errors represent the differing capabilities of human participants in executing tasks as per the instructions (decision tree) provided. And $\beta_j$ is used to  represent other unknown factors. For example, some participants may device their own heuristic based on the experience they gain from completing several tasks.
    Let $m_d\coloneqq m_B-m_O.$ The hypothesis can be defined as follows.
    \begin{align}
        \Hyp_{B}: m_{d}=0,\nonumber\\
        \Hyp_{O}: m_{d}>0.
    \end{align}
    Notice that in the above formulation the unknown additive effect $\beta_j$ cancels out. A single sample $t$-test is conducted with the following test statistic.
    \begin{align}
        &t_0 = \frac{\bar{d}}{S_d/\sqrt{n}},\nonumber\\
        &\bar{d} = \frac{1}{n}\sum\limits_{j=1}^{n}d_j,\nonumber\\
        &S_d = \frac{1}{n-1}\left[\sum\limits_{j=1}^{n}(d_j-\bar{d})^2 \right]^{1/2},
    \end{align}
    where $d_j\coloneqq y^B_j-y^O_j.$ Hypothesis $\Hyp_B$ can be rejected if $\lvert t_0 \rvert$ is greater than a threshold. This is called a paired $t$-test.
    This assumes that the variances of random errors of the both treatment groups are the same.
    %\begin{align}
    %    \Hyp_{B}: m_{B}=m_{O},\nonumber\\
    %    \Hyp_{O}: m_{B}>m_{O}.
    %\end{align}
    %
    %\begin{align}
    %    \Hyp_{B}: v_{B}=v_{O},\nonumber\\
    %    \Hyp_{O}: v_{B}>v_{O}.
    %\end{align}
    
    \item \textit{Randomization ---} We use the paired comparison design where for each experimental unit both the treatments are applied in random order. This allows for neutralizing any bias that may creep due to the ``haphazard'' arrival of the participants.
    
    \item \textit{Choice of sample size ---} We can choose the sample size based on the operating characteristic (OC) curve or power curve for the statistical test. A detailed analysis of the considerations for choosing sample sizes can be found in Chapter $2$ of \cite{Montgomery:book2017:DAE}. We choose $20$ samples using conservative estimates (obtained from previous simulations) of the difference in mean costs $m_B-m_O$ while assuming $v_B=V_O.$

    \item \textit{Responses ---} These are outcomes that are observed upon applying the  treatments/allocation schemes to the experimental units. Our experiment setup ``measures'' all the classification decisions made by the human participants under different allocation schemes. These measurements are 
    used to compute the sample mean of the cost per batch of tasks and sample variance of cost per batch of tasks which represent the response of each experimental unit.
    These can be called \textit{surrogate responses} as they are only measured for the specific type of classification problem provided by our experimental setup. However, we will use these \textit{surrogate responses} to judge the performance of various allocation schemes and apply it to situations which satisfy our modeling assumptions.
    %where  classification performance degrades with workload.
    This extrapolation of our judgement requires that the surrogate responses are good predictors of responses in the other situations. 

    \item \textit{Experimental error ---} There is random variation in the responses of experimental units to the same allocation scheme. The same allocation scheme may have variation in response of an experimental unit if applied over and over again. The model for this error is described in the following.

\end{enumerate}
